# Supplementary material for: Differentially Private Publication of Location Entropy
Source: arXiv:1909.00882 source file (2019-09-02)
Supplement: Supplementary file 1 [file appendix.tex]

\appendix
\section{Proof of Theorem}

\subsection{Proof of Theorem~\ref{theorem:globalBoundOfDeltaH}}
\label{sec:all_location}

We prove the bound of global sensitivity for two cases, $c = 1$ and $c > 1$.
It is obvious that when $c = 1$, the maximum of the change of location entropy is $\log 2$.

When $c > 1$, $\log (1 + \dfrac{1}{\exp(H(\mathcal{C} \setminus c_u))})$ decreases when $n$ increases. 
Thus, it is maximized when $n = 1$ and the maximum change is $\log 2$.

We also have:
\begin{displaymath}
\begin{split}
& \quad \Big(\log \frac{n - 1}{n - 1 + C} + \frac{C}{n - 1 + C} \log C \Big)'_n \\
&= \frac{1}{n - 1} - \frac{1}{n - 1 + C} - \frac{C\log C}{(n - 1 + C)^2} \\
&= \frac{(n - 1 + C)^2 - (n - 1)(n - 1 + C) - (n - 1)C\log C}{(n - 1)(n - 1 + C)^2} \\
&= \frac{C^2 + (n - 1)C - (n - 1)C\log C}{(n - 1)(n - 1 + C)^2} \\
\end{split}
\end{displaymath}

\begin{displaymath}
\begin{split}
& \quad \Big(\log \frac{n - 1}{n - 1 + C} + \frac{C}{n - 1 + C} \log C \Big)'_n \ge 0\\
&\Leftrightarrow C^2 + (n - 1)C - (n - 1)C\log C \ge 0 \\
&\Leftrightarrow C \ge (n - 1)(\log C - 1)
\end{split}
\end{displaymath}

If $\log C - 1 \ge 0$ or $C$ is not less than the base of the logarithm (which is $\mathrm{e}$ in this work),
where $n = \frac{C}{\log C - 1} + 1$, $\log \frac{n - 1}{n - 1 + C} + \frac{C}{n - 1 + C} \log C$ is maximized and:
\begin{displaymath}
\begin{split}
& \quad \log \frac{n - 1}{n - 1 + C} + \frac{C}{n - 1 + C} \log C \\
&= \log \Big(\frac{\dfrac{C}{\log C - 1}}{\dfrac{C}{\log C - 1} + C} \Big) + \frac{C}{\dfrac{C}{\log C - 1} + C} \log C\\
&= \log \frac{C}{C + C\log C - C} + \frac{C(\log C - 1)\log C}{C\log C}\\
&= \log \frac{1}{\log C} + \log C - 1\\
&= \log C - \log (\log C) - 1\\
\end{split}
\end{displaymath}

If $\log C - 1 < 0$, $\log \frac{n - 1}{n - 1 + C} + \frac{C}{n - 1 + C} \log C$ always increases. We have:
\begin{displaymath}
\lim_{n \to \infty} \frac{n - 1}{n - 1 + C} + \frac{C}{n - 1 + C} \log C = 0
\end{displaymath}
\begin{displaymath}
\Rightarrow \frac{n - 1}{n - 1 + C} + \frac{C}{n - 1 + C} \log C < 0
\end{displaymath}

Similarly, we can prove that:
\begin{displaymath}
\max_n \Big( \log \frac{n}{n + C} + \frac{C}{n + C} \log C \Big) = \log C - \log (\log C) - 1 
\end{displaymath}

\subsection{Proof of Theorem~\ref{theorem:boundOfDeltaH}}
\label{sec:one_location}

In this section, we derive the bound for the sensitivity of location entropy of a particular location $l$ when the data of a user is removed from the dataset.

For convenience, let $n$ be the number of users visiting $l$, $n=|U_l|$, $c_u = |O_{l,u}|$. Let $\mathcal{C} = \{c_1, c_2, \dots, c_n\}$ be the set of numbers of visits of all users to location $l$.
Let $S = |O_l| = \sum_{u} c_u$.
Let $S_u = S - c_u$ be the sum of numbers of visits of all users to location $l$ after removing user $u$.
From Equation~\ref{eq:le}, we have:
\begin{displaymath}
H(l)=H(O_l) = H(\mathcal{C}) = - \sum_{u} \frac{c_u}{S} \log \frac{c_u}{S}  \nonumber
\end{displaymath}
By removing a user $u$, entropy of location $l$ becomes:
\begin{displaymath}
H(\mathcal{C} \setminus c_u) = - \sum_{u} \frac{c_u}{S_u} \log \frac{c_u}{S_u}
\end{displaymath}
From Equation~\ref{eq:entropy_add}, we have:
\begin{displaymath}
H(\mathcal{C}) = \frac{S_u}{S} H(\mathcal{C} \setminus c_u) + H(\frac{S_u}{S}, \frac{c_u}{S})
\end{displaymath}
Subsequently, the change of location entropy when a user $u$ is removed is:
\begin{equation}
\label{eq:deltaH}
\Delta H_u = H(\mathcal{C} \setminus c_u) - H(\mathcal{C}) \\
= \frac{c_u}{S} H(\mathcal{C} \setminus c_u) - H(\frac{S_u}{S}, \frac{c_u}{S})
\end{equation}

Taking derivative of $\Delta H_u$ w.r.t $c_u$:
\begin{displaymath}
\begin{split}
(\Delta H_u)'_{c_u}	&= \frac{S - c_u}{S^2} H(\mathcal{C} \setminus c_u) + (\frac{S_u}{S} \log \frac{S_u}{S} + \frac{c_u}{S} \log \frac{c_u}{S})'_{c_u} \\
							&= \frac{S_u}{S^2} H(\mathcal{C} \setminus c_u) - \frac{S_u}{S^2} \log \frac{S_u}{S} + \frac{S_u}{S} \frac{-\dfrac{S_u}{S^2}}{\dfrac{S_u}{S}} \\
							& \quad + \frac{S_u}{S^2} \log \frac{c_u}{S} + \frac{c_u}{S} \frac{\dfrac{S_u}{S^2}}{\dfrac{c_u}{S}} \\
							&= \frac{S_u}{S^2} H(\mathcal{C} \setminus c_u) - \frac{S_u}{S^2} \log \frac{S_u}{S} - \frac{S_u}{S^2} + \frac{S_u}{S^2} \log \frac{c_u}{S} + \frac{S_u}{S^2} \\
							&= \frac{S_u}{S^2} (H(\mathcal{C} \setminus c_u) - \log \frac{S_u}{c_u})
\end{split}
\end{displaymath}

We have: 
\begin{displaymath}
\begin{split}
(\Delta H_u)'_{c_u}	= 0 \Leftrightarrow H(\mathcal{C} \setminus c_u) = \log \frac{S_u}{c_u}
\end{split}
\end{displaymath}

Therefore, $\Delta H_u$ decreases when $c_u \le c^*_u$, and increases when $c^*_u < c_u$ 
where $c^*_u$ is the value so that $H(\mathcal{C} \setminus c_u) = \log \frac{S_u}{c^*_u}$. 

In addition, because $H(\mathcal{C} \setminus c_u) \le log (n-1)$ and $n - 1 < S_u$ when $C > 1$, \newline
$\Rightarrow$  $\Delta H_u < 0$ when $c_u = 1$ \newline
$\Rightarrow$  $|\Delta H_u|$ is maximized when $c_u = c^*_u$ or $c_u = C$. 

\textbf{Case 1:} $c_u = C$: 

If $\Delta H_u < 0$, $|\Delta H_u|$ is maximized when $c_u = c^*_u$.

If $\Delta H_u > 0$, we have:
\begin{displaymath}
\begin{split}
0	&\le \frac{c_u}{S} H(\mathcal{C} \setminus c_u) - H(\frac{S_u}{S}, \frac{c_u}{S}) \\
	&\le \frac{C}{S} \log (n - 1) - H(\frac{S_u}{S}, \frac{C}{S}) \\
\end{split}
\end{displaymath}

Taking the derivative of the right side w.r.t $S_u$:
\begin{displaymath}
\begin{split}
&\Big( \frac{C}{S} \log (n - 1) - H(\frac{S_u}{S}, \frac{C}{S}) \Big)'_{S_u} \\
&=\Big( \frac{C}{S_u + C} \log (n - 1) - H(\frac{S_u}{S_u + C}, \frac{C}{S_u + C}) \Big)'_{S_u} \\
&=\Big( \frac{C}{S_u + C} \log (n - 1) + \frac{S_u}{S_u + C} \log \frac{S_u}{S_u + C} + \frac{C}{S_u + C} \log \frac{C}{S_u + C} \Big)'_{S_u} \\
&=\frac{-C}{(S_u + C)^2} \log (n - 1) + \frac{C}{(S_u + C)^2} \log \frac{S_u}{S_u + C} + \frac{C}{(S_u + C)^2} \\
& \quad - \frac{C}{(S_u + C)^2} \log \frac{C}{S_u + C} - \frac{C}{(S_u + C)^2} \\
&=\frac{C}{(S_u + C)^2} \Big( -\log (n - 1) + \log \frac{S_u}{C} \Big) \\
&=\frac{C}{(S_u + C)^2} \log \frac{S_u}{(n - 1) C} \\
&\le 0
\end{split}
\end{displaymath}

$\Rightarrow$ $\Delta H_u$ is maximized when $S_u$ is minimized.

$\Rightarrow$ When $c_u = C$ and  $\Delta H_u > 0$:
\begin{displaymath}
\begin{split}
\Delta H_u		&\le \frac{C}{n - 1 + C} \log (n - 1) - H(\frac{n-1}{n - 1 + C}, \frac{C}{n - 1 + C}) \\
					&= \frac{C}{n - 1 + C} \log (n - 1) + \frac{n-1}{n - 1 + C} \log \frac{n-1}{n - 1 + C} \\
					& \quad + \frac{C}{n - 1 + C} \log \frac{C}{n - 1 + C} \\
					&= \log \frac{n - 1}{n - 1 + C} + \frac{C}{n - 1 + C} \log C
\end{split}
\end{displaymath}

\textbf{Case 2:} $c_u = c^*_u$:
\begin{displaymath}
\begin{split}
\Delta H_u		&= \frac{c_u}{S} \log \frac{S_u}{c_u} - H(\frac{S_u}{S}, \frac{c_u}{S}) \\
					&= \frac{c_u}{S} \log \frac{S_u}{c_u} + \frac{S_u}{S} \log \frac{S_u}{S} + \frac{c_u}{S} \log \frac{c_u}{S} \\
					&= \frac{c_u}{S} \log \frac{S_u}{S} + \frac{S_u}{S} \log \frac{S_u}{S} \\
					&= \log \frac{S_u}{S} \\
					&= -\log \frac{S}{S_u} \\
					&= -\log \frac{S_u + c_u}{S_u} \\
					&= -\log (1 + \frac{c_u}{S_u}) \\
					&= -\log (1 + \frac{1}{\frac{S_u}{c_u}}) \\
					&= -\log (1 + \frac{1}{\exp(H(\mathcal{C} \setminus c_u))}) \\
\end{split}
\end{displaymath}

$\Rightarrow$ $\Delta H_u$ is maximized when $H(\mathcal{C} \setminus c_u)$ is minimized.

\begin{lemma} %
\label{lemma:minimumEntropy}
Given a set of $n$ numbers, $\mathcal{C} = \{c_1, c_2, \dots, c_n\}$, 
$1 \le c_i \le C$,
entropy $H(\mathcal{C})$ is minimized when $c_i = 1$ or $c_i = C$, for all $i = 1,\dots,n$.
\end{lemma}

\begin{proof}
When the value of a number $c_u$ is changed and others a fixed, from \hyperref[eq:deltaH]{equation~\ref{eq:deltaH}}:
\begin{displaymath}
\begin{split}
H(\mathcal{C})'_{c_u}		&= (\Delta H_u)'_{c_u} \\
									&= \frac{S_u}{S^2} (\log \frac{S_u}{c_u} - H(\mathcal{C} \setminus c_u)) \\
\end{split}
\end{displaymath}

Therefore, $H(\mathcal{C})$ increases when $c_u \le c^*_u$, and decreases when $c^*_u < c_u$ 
where $c^*_u$ is the value so that $H(\mathcal{C} \setminus c_u) = \log \frac{S_u}{c^*_u}$.

$\Rightarrow$ $H(\mathcal{C})$ is minimized when $c_u = 1$ or $c_u = C$.

\end{proof}

\begin{lemma} [Minimum Entropy]
\label{lemma:minimumEntropyValue}
Given a set of $n$ numbers, $\mathcal{C} = \{c_1, c_2, \dots, c_n\}$, 
$1 \le c_i \le C$, 
the minimum entropy $H(\mathcal{C}) = \log n - \frac{\log C}{C - 1} + \log \Big( \frac{\log C}{C - 1} \Big) + 1$.
\end{lemma}

\begin{proof}
Using \hyperref[lemma:minimumEntropy]{Lemma~\ref{lemma:minimumEntropy}}, entropy $H(\mathcal{C})$ is minimized when 
$\mathcal{C} = \{\underbrace{1, \dots, 1}_{\mathclap{n - k  \text{ times}}}, \underbrace{C, \dots, C}_{\mathclap{k \text{ times}}} \}$.

Let $S = \sum_i c_i = n - k + kC$. We have:
\begin{displaymath}
\begin{split}
H(\mathcal{C})	&= - \frac{n-k}{S} \log \frac{1}{S} - \frac{kC}{S} \log \frac{C}{S} \\
						&= \frac{n-k}{S}\log S + \frac{kC}{S} \log S - \frac{kC}{S}\log C \\
						&= \log S - \frac{k C}{S} \log C \\
\end{split}
\end{displaymath}

We have $S'_k = C - 1$.
Take the derivative of $H(\mathcal{C})$ w.r.t $k$, we have:
\begin{displaymath}
\begin{split}
(H(\mathcal{C}))'_k		&= \frac{C - 1}{S} - \frac{S - k(C - 1)}{S^2} C \log C \\
								&= \frac{1}{S^2} \Big( S(C - 1) - (S - kC + k)C \log C \Big)\\
								&= \frac{1}{S^2} \Big((n - k + kC)(C - 1) - (n - k + kC - kC + k)C \log C \Big)\\
								&= \frac{1}{S^2} (nC - n - kC + k + k C^2 - kC - nC \log C)\\
\end{split}
\end{displaymath}

$(H(\mathcal{C}))'_k	 = 0 \Leftrightarrow k = \dfrac{n(C \ log C - C + 1)}{(C - 1)^2}$

When $k = 0$ or $k = n$, $H(\mathcal{C})$ is maximized.
Thus $H(\mathcal{C})$ is minimized when $k = \dfrac{n(C \ log C - C + 1)}{(C - 1)^2}$.
It is clear that we need $k$ to be an integer. 
Thus, $k$ would be chosen as $\floor*{k}$ or $\floor*{k} + 1$, depending on what value creates a smaller value of $H(\mathcal{C})$. 

\begin{displaymath}
\begin{split}
S	&= n - k + kC \\
	&= n + k(C - 1) \\
	&= n + \frac{n(C \ log C - C + 1)}{C - 1} \\
	&= \frac{nC - n + nC\log C - nC + n}{C - 1} \\
	&= \frac{nC\log C}{C - 1}
\end{split}
\end{displaymath}

\begin{displaymath}
\begin{split}
\frac{kC}{S} \log C	&= \frac{n(C \ log C - C + 1)}{(C - 1)^2} C \frac{C - 1}{nC\log C} \log C\\
							&= \frac{C\log C - C + 1}{C - 1}
\end{split}
\end{displaymath}

\begin{displaymath}
\begin{split}
H(\mathcal{C})	&= \log \Big( \frac{nC\log C}{C - 1} \Big) - \frac{C\log C - C + 1}{C - 1} \\
						&= \log n + \log \Big( \frac{C\log C}{C - 1} \Big) - \frac{C\log C}{C - 1} + 1 \\
						&= \log n - \frac{\log C}{C - 1} + \log \Big( \frac{\log C}{C - 1} \Big) + 1
\end{split}
\end{displaymath}
\end{proof}

Using \hyperref[lemma:minimumEntropyValue]{Lemma~\ref{lemma:minimumEntropyValue}}, when $c_u = c^*_u$:
\begin{displaymath}
|\Delta H_u|		\le \log (1 + \frac{1}{\exp(H(\mathcal{C} \setminus c_u))})
\end{displaymath}
where $H(\mathcal{C} \setminus c_u) = \log (n-1) - \frac{\log C}{C - 1} + \log \Big( \frac{\log C}{C - 1} \Big) + 1$.

Thus, the maximum change of location entropy when a user is \textit{removed} equals :

\begin{itemize}
\item $\log \frac{n}{n-1}$ when $C = 1$
\item 
$\max\Big(\log \frac{n - 1}{n - 1 + C} + \frac{C}{n - 1 + C} \log C,  \log (1 + \frac{1}{\exp(H(\mathcal{C} \setminus c_u))}) \Big)$
where $H(\mathcal{C} \setminus c_u) = \log (n-1) - \frac{\log C}{C - 1} + \log \Big( \frac{\log C}{C - 1} \Big) + 1$,
when $n > 1, c > 1$.
\end{itemize}

Similarly, the maximum change of location entropy when a user is \textit{added} equals :

\begin{itemize}
\item $\log \frac{n+1}{n}$ when $C = 1$
\item 
$\max\Big(\log \frac{n}{n + C} + \frac{C}{n + C} \log C,  \log (1 + \frac{1}{\exp(H(\mathcal{C} \setminus c_u))}) \Big)$
where $H(\mathcal{C} \setminus c_u) = \log (n-1) - \frac{\log C}{C - 1} + \log \Big( \frac{\log C}{C - 1} \Big) + 1$,
when $n > 1, c > 1$.
\end{itemize}

Thus, we have the proof for \hyperref[theorem:boundOfDeltaH]{Theorem~\ref{theorem:boundOfDeltaH}}.

\subsection{Proof of Theorem~\ref{theorem:privacyGuarantee}}
\label{sec:proof_limit}

In this section, we prove that Theorem~\ref{theorem:privacyGuarantee} satisfies $\epsilon$-differential privacy. We prove the theorem when a user is removed from the database. The case when a user is added is similar.

Let $l$ be an arbitrary location and $\mathcal{A}_l: L \rightarrow \mathbb{R}$  be the \hyperref[alg:baseline]{Algorithm~\ref{alg:limit}} when only location $l$ is considered for perturbation.
$O_{l\text{(org)}}$ be the original set of observations at location $l$; 
$O_{l, u\text{(org)}}$ be the original set of observations of user $u$ at location $l$; 
$O_{l, u}$ be the set of observations after limiting $c_{u}$ to $C$ and limiting maximum $M$ locations per user;
$O_l$ be the set of all $O_{l, u}$ for all users $u$ that visit location $l$;
$\mathcal{C}$ be the set visits.
Let $O_l \setminus O_{l,u}$ be the set of observations at location $l$ when a user $u$ is removed from the dataset.
Let $b = \frac{M \Delta H}{\epsilon}$.

If $O_{l, u\text{(org)}} = \varnothing$:
\begin{displaymath}
\frac{Pr[\mathcal{A}_l(O_{l\text{(org)}}) = t_l]}{Pr[\mathcal{A}_l(O_{l\text{(org)}} \setminus O_{l, u\text{(org)}}) = t_l]} = 1 
\end{displaymath}

If $O_{l, u\text{(org)}} \neq \varnothing$:
\begin{displaymath}
\begin{split}
& \quad \frac{Pr[\mathcal{A}_l(O_{l\text{(org)}}) = t_l]}{Pr[\mathcal{A}_l(O_{l\text{(org)}} \setminus O_{l, u\text{(org)}}) = t_l]} \\
&= \frac{Pr[\mathcal{A}_l(O_l) = t_l]}{Pr[\mathcal{A}_l(O_l \setminus O_{l,u}) = t_l]}  \\
&= \frac{Pr[H(\mathcal{C}) + \text{Lap}(b) = t_l]}{Pr[H(\mathcal{C} \setminus c_{l,u}) + \text{Lap}(b) = t_l]} \\
\end{split}
\end{displaymath}

If $H(\mathcal{C}) \le H(\mathcal{C} \setminus c_{l,u})$:
\begin{displaymath}
\begin{split}
& \quad \frac{Pr[H(\mathcal{C}) + \text{Lap}(b) = t_l]}{Pr[H(\mathcal{C} \setminus c_{l,u}) + \text{Lap}(b) = t_l]} \\
&= \frac{Pr[H(\mathcal{C}) + \text{Lap}(b) = t_l]}{Pr[H(\mathcal{C}) + \Delta H(l) + \text{Lap}(b) = t_l]} \\
&= \frac{Pr[\text{Lap}(b) = t_l - H(\mathcal{C})]}{Pr[\text{Lap}(b) = t_l - H(\mathcal{C}) - \Delta H(l)]} \\
&= \exp \Big(\frac{1}{b} (-|t_l - H(\mathcal{C})| + |t_l - H(\mathcal{C}) - \Delta H(l)|) \Big) \\
&\le \exp(\frac{|\Delta H(l)|}{b})  \\
&\le \exp(\frac{\Delta H}{b})  \\
&= \exp(\frac{\epsilon}{M}) \\
\end{split}
\end{displaymath}

If $H(\mathcal{C}) > H(\mathcal{C} \setminus c_{l,u})$, similarly:
\begin{displaymath}
\frac{Pr[H(\mathcal{C}) + \text{Lap}(b) = t_l]}{Pr[H(\mathcal{C} \setminus c_{l,u}) + \text{Lap}(b) = t_l]} \le \exp(\frac{\epsilon}{M}) \\
\end{displaymath}

Similarly, we can prove that:
\begin{displaymath}
\frac{Pr[\mathcal{A}_l(O_{l\text{(org)}} \setminus O_{l, u\text{(org)}}) = t_l]}{Pr[\mathcal{A}_l(O_{l\text{(org)}}) = t_l]} \le exp(\frac{\epsilon}{M})
\end{displaymath}

Therefore, $\mathcal{A}_l$ satisfies $0$-differential privacy when $O_{l, u\text{(org)}} = \varnothing$, and satisfies $\frac{\epsilon}{M}$-differential privacy when $O_{l, u\text{(org)}} \neq \varnothing$.

For all locations, let $\mathcal{A}: L \rightarrow \mathbb{R}^{|L|}$  be the \hyperref[alg:baseline]{Algorithm~\ref{alg:limit}}. let $L_1$ be any subset of $L$.
Let $T = \{t_1, t_2, \dots, t_{|L_1|}\} \in $\textit{Range}($\mathcal{A}$) denote an arbitrary possible output.
Thus, $\mathcal{A}$ is the composition of all $\mathcal{A}_l$, $l \in L$.
Let $L(u)$ be the set of all locations that $u$ visits, $|L(u)| \le M$.
Applying composition theorems~\cite{dwork2014algorithmic} for all $\mathcal{A}_l$ where $\mathcal{A}_l$ satisfies $0$-differential privacy when $l \notin L_1 \cap L(u)$, and satisfies $\frac{\epsilon}{M}$-differential privacy when $l \in L_1 \cap L(u)$, we have $\mathcal{A}$ satisfies $\epsilon$-differential privacy.
